# Supplementary material for: A four parameter model for the solid-electrolyte interphase to predict battery aging during operation
Source: arXiv:2112.13671 ancillary file (2022-11-30)
Supplement: Supplementary file 1 [file Supporting_Information_revised.pdf]

# Supporting Information
# A four parameter model for the solid-electrolyte interphase to predict battery aging during operation


Lars von Kolzenberg *[1,2], Jochen Stadler =[3,4], Johannes Fath[4], Madeleine Ecker[4], Birger Horstmann[1,2,3], and Arnulf Latz †[1,2,3]

[1]German Aerospace Center, Pfaffenwaldring 38-40, 70569 Stuttgart, Germany
[2]Helmholtz Institute Ulm, Helmholtzstraße 11, 89081 Ulm, Germany
[3]Ulm University, Albert-Einstein-Allee 47, 89081 Ulm, Germany
[4]Mercedes-Benz AG, Mercedesstr. 120, 70372 Stuttgart, Germany



November 30, 2022


## 1 Experimental Details

Figure SI-1 shows the OCV-curve of the full cell, anode and cathode at the begin of life, which sets the basis for our differential voltage analysis.

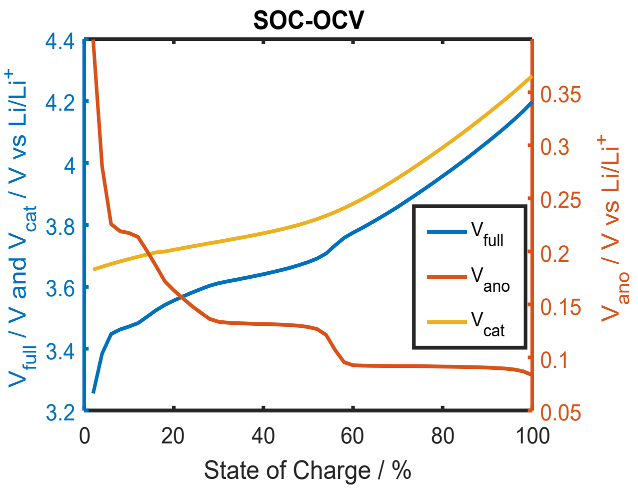


Figure SI-1: Pseudo OCV of full cell, anode and cathode. Measured with three-electrode cell setup with material taken from pouch cell at begin of life.

In Table SI-1, we list the 28 different aging conditions of the 62 cells. The color codes the respective values from lowest (green) over intermediate (yellow) to highest (red).


*These authors contributed equally to this work
†Corresponding Author: arnulf.latz@dlr.de

| Test-No. | Cell-No. | Temp / [°C] | $SoC_{max}$ /[%] | $SoC_{min}$ / [%] | $EV_{ratio}$ / [%] | $P_{CH}$ / [W] |
|---|---|---|---|---|---|---|
| 1 | 1 | 22 | 86 | 25 | 80 | 72 |
| 1 | 2 | 22 | 86 | 24 | 80 | 72 |
| 2 | 23 | 39 | 85 | 23 | 40 | 72 |
| 2 | 24 | 39 | 85 | 23 | 40 | 72 |
| 3 | 49 | 21 | 95 | 26 | 40 | 72 |
| 3 | 50 | 21 | 96 | 26 | 40 | 72 |
| 4 | 51 | 39 | 95 | 25 | 80 | 72 |
| 4 | 52 | 39 | 95 | 26 | 80 | 72 |
| 5 | 53 | 20 | 86 | 32 | 40 | 72 |
| 5 | 54 | 20 | 86 | 32 | 40 | 72 |
| 6 | 55 | 41 | 86 | 32 | 80 | 72 |
| 6 | 56 | 41 | 86 | 32 | 80 | 72 |
| 7 | 57 | 22 | 96 | 30 | 80 | 72 |
| 7 | 58 | 22 | 96 | 34 | 80 | 72 |
| 8 | 59 | 41 | 95 | 33 | 40 | 72 |
| 8 | 60 | 41 | 95 | 33 | 40 | 72 |
| 9 | 61 | 21 | 86 | 24 | 40 | 200 |
| 9 | 62 | 21 | 86 | 24 | 40 | 200 |
| 10 | 3 | 39 | 86 | 24 | 80 | 200 |
| 10 | 4 | 40 | 86 | 24 | 80 | 200 |
| 11 | 5 | 21 | 96 | 26 | 80 | 200 |
| 11 | 6 | 21 | 96 | 25 | 80 | 200 |
| 12 | 7 | 41 | 95 | 26 | 40 | 200 |
| 12 | 8 | 41 | 95 | 26 | 40 | 200 |
| 13 | 9 | 21 | 86 | 32 | 80 | 200 |
| 13 | 10 | 22 | 86 | 32 | 80 | 200 |
| 14 | 11 | 41 | 86 | 32 | 40 | 200 |
| 14 | 12 | 41 | 86 | 32 | 40 | 200 |
| 15 | 13 | 22 | 92 | 32 | 40 | 200 |
| 15 | 14 | 22 | 96 | 33 | 40 | 200 |
| 16 | 15 | 41 | 95 | 33 | 80 | 200 |
| 16 | 16 | 41 | 95 | 34 | 80 | 200 |
| 17 | 17 | 11 | 92 | 29 | 60 | 136 |
| 17 | 18 | 11 | 92 | 29 | 60 | 136 |
| 18 | 19 | 50 | 90 | 29 | 60 | 136 |
| 18 | 20 | 50 | 87 | 28 | 60 | 136 |
| 19 | 21 | 30 | 81 | 27 | 60 | 136 |
| 19 | 22 | 31 | 81 | 27 | 60 | 136 |
| 20 | 25 | 30 | 100 | 30 | 60 | 136 |
| 20 | 26 | 30 | 100 | 30 | 60 | 136 |
| 21 | 27 | 30 | 90 | 21 | 60 | 136 |
| 21 | 28 | 30 | 90 | 21 | 60 | 136 |
| 22 | 29 | 31 | 91 | 37 | 60 | 136 |
| 22 | 30 | 31 | 91 | 37 | 60 | 136 |
| 23 | 31 | 31 | 90 | 28 | 60 | 8 |
| 23 | 32 | 31 | 90 | 28 | 60 | 8 |
| 24 | 33 | 31 | 90 | 29 | 60 | 264 |
| 24 | 34 | 31 | 90 | 29 | 60 | 264 |
| 25 | 35 | 31 | 90 | 28 | 20 | 136 |
| 25 | 36 | 31 | 90 | 29 | 20 | 136 |
| 26 | 37 | 29 | 91 | 29 | 100 | 136 |
| 26 | 38 | 29 | 91 | 29 | 100 | 136 |

| | | | | | | |
|---|---|---|---|---|---|---|
| 27 | 39 | 31 | 90 | 29 | 60 | 136 |
| 27 | 40 | 30 | 90 | 28 | 60 | 136 |
| 27 | 41 | 30 | 90 | 29 | 60 | 136 |
| 27 | 42 | 30 | 90 | 29 | 60 | 136 |
| 27 | 43 | 30 | 91 | 29 | 60 | 136 |
| 27 | 44 | 31 | 90 | 29 | 60 | 136 |
| 27 | 45 | 31 | 90 | 29 | 60 | 136 |
| 27 | 46 | 31 | 90 | 28 | 60 | 136 |
| 28 | 47 | 30 | 48 | 48 | 0 | |
| 28 | 48 | 30 | 47 | 47 | 0 | |

Table SI-1: Cyclic Aging Conditions with color coding from lowest (green) to highest (red) level of each factor. Test 28 is pure calendar aging.

## 2 Computational Details

In this section, we discuss the computational details to numerically evaluate our model and discuss our approach to obtain the free parameters. Initially, we fit the initial SEI thickness $L_{\mathrm{SEI},0}$ and the prefactor $c_{\mathrm{e}^-,0}D_{\mathrm{e}^-,0}$ to storage experiments with a least-square fitting routine implemented in MATLAB's *lsqcurvefit*. The active lithium inventory $1 - Q_{\mathrm{LL}}/Q_{\mathrm{max}}$ results from the SEI thickness with Equation 4.

With these parameters, we proceed to simulate SEI growth during battery cycling. First, we determine the state of charge $\tilde{c}$ by integrating the applied current $\tilde{J}$ over time, according to Equation 9. Then, we obtain the overpotential $\tilde{\eta}_{\mathrm{SEI}}$ from the state of charge $\tilde{c}$ and the current $\tilde{J}$ with Equation 8. Finally, we numerically solve Equation 10 with a trapezoidal integration rule implemented in MATLAB's *trapz* leading to the SEI growth $L_{\mathrm{SEI}}(\tilde{t})$.

Evaluating Equation 10 requires additional fitting parameters to determine the current and temperature dependence of aging. For the current dependence, we adapt the intercalation exchange current $J_{\mathrm{int},0,0}$ of Equation 2 to fit the center cells (39-46), which were measured eight fold and thus show the lowest experimental uncertainty. For the temperature dependence, we manually fit the exponent $\mu_{\mathrm{e}^-,0} + E_{\mathrm{A}}$ of Equation 7 and 8 to the high temperature cells (19,20). The parameters used and obtained in this process are listed in Table SI-2.

Based on this parametrization, we proceed to validate our model with the remaining cells. As measure for the goodness of fit, we use the root-mean-square error defined as

$$\mathrm{RMSE} = \frac{1}{n}\sqrt{\sum_{i=1}^{n}(\hat{y}_i - y_i)^2} \qquad \text{(SI-1)}$$

with the model predictions $\hat{y}_i$ of the experimental values $y_i$.

Regarding the experimental values $y_i$, we made two restrictions to increase the comparability of our results and point out the predictivity of our model. First, we restricted our RMSE calculation to the 25 validation protocols, which were not used to parametrize the model. Second, we used only the data of the first of the twin cells per protocol. This cell was stopped after around 2.5 years to perform post-mortem analysis. Concludingly, our experimental data thus comprises one cell per validation protocol with capacity measurements performed every 2 weeks for around 2.5 years amounting to $n = 918$ datapoints. Figure SI-2 shows the evolution of the RMSE with increasing lithium loss.

In Figure SI-3, we show the full model evaluation and compare the predicted capacity fade with the experiments in the landscape figure.

## References


[1] Fabian Single, Arnulf Latz, and Birger Horstmann. Identifying the Mechanism of Continued Growth of the Solid–Electrolyte Interphase. *ChemSusChem*, 11(12):1950–1955, 2018.

| Description | Variable | Value | Source |
|---|---|---|---|
| Faraday's constant | $F$ | $96\,485\,\mathrm{C\,mol^{-1}}$ | |
| Universal gas constant | $R$ | $8.314\,\mathrm{J\,mol^{-1}\,K^{-1}}$ | |
| Electrode active surface | $A$ | $233.4\,\mathrm{m^2}$ | Estimated from [1] |
| Maximum battery capacity | $Q_{\mathrm{max}}$ | $45.89\,\mathrm{A\,h}$ | Experimental data |
| OCV curve | $U_0(\tilde{c})$ | Figure SI-1 | Experimental data |
| Molar Volume of SEI components | $V_{\mathrm{SEI}}$ | $96.2 \cdot 10^{-6}\,\mathrm{m^3\,mol^{-1}}$ | [2] |
| Stoichiometry of e$^-$, 0 in Reaction 3 | $\nu_{\mathrm{SEI}}$ | 2 | |
| Reference concentration of lithium atoms | $c_{\mathrm{e^-},0}$ | $1 \cdot 10^{-3}\,\mathrm{mol\,m^{-3}}$ | Assumed |
| Initial SEI thickness | $L_{\mathrm{SEI},0}$ | $3.9\,\mathrm{nm}$ | Fitted to cells 47,48 |
| Interstitial reference chemical potential | $\mu_{\mathrm{e^-},0}$ | 0 | Gauged to lithium metal |
| Intercalation reaction rate | $J_{\mathrm{int},0,0}$ | $21\,\mathrm{A}$ | Fitted to cells 39-46 |
| Reference diffusivity of lithium atoms | $D_{\mathrm{e^-},0}$ | $1.26 \cdot 10^{-12}\,\mathrm{m^2\,s^{-1}}$ | Fitted to cells 19,20 and 47,48 |
| Diffusion activation energy | $E_{\mathrm{A}}$ | $13.25\,\mathrm{kJ\,mol^{-1}}$ | Fitted to cells 19,20 and 47,48 |
| Intercalated charge | $Q_{\mathrm{int}}$ | | |
| Intercalation current | $J_{\mathrm{int}}$ | | |
| Time | $t$ | | |
| Intercalation overpotential | $\eta_{\mathrm{int}}$ | | |
| Intercalation exchange current | $J_{\mathrm{int},0}$ | | |
| Lost lithium inventory | $Q_{\mathrm{LL}}$ | | |
| SEI thickness | $L_{\mathrm{SEI}}$ | | |
| SEI formation current density | $j_{\mathrm{SEI}}$ | | |
| Lithium interstitial diffusivity | $D_{\mathrm{Li},0}$ | | |
| Lithium interstitial formation overpotential | $\eta_{\mathrm{SEI}}$ | | |
| State of charge | $\tilde{c}$ | | |

Table SI-2: Parameter implemented in the simulation and list of symbols

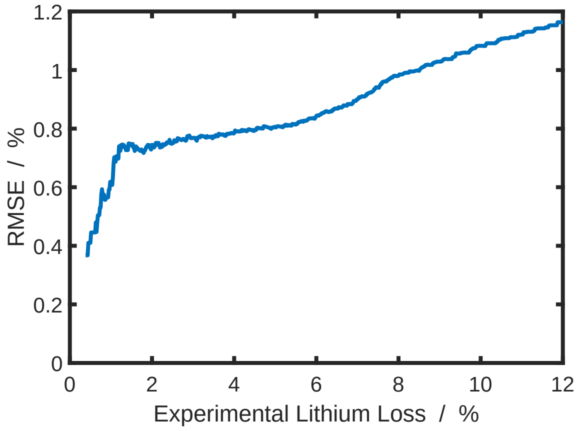


Figure SI-2: Root mean squared error RMSE, Equation SI-1, depending on the loss of active lithium.

[2] Oleg Borodin, Grant D. Smith, and Peng Fan. Molecular dynamics simulations of lithium alkyl carbonates. *Journal of Physical Chemistry B*, 110(45):22773–22779, 2006.

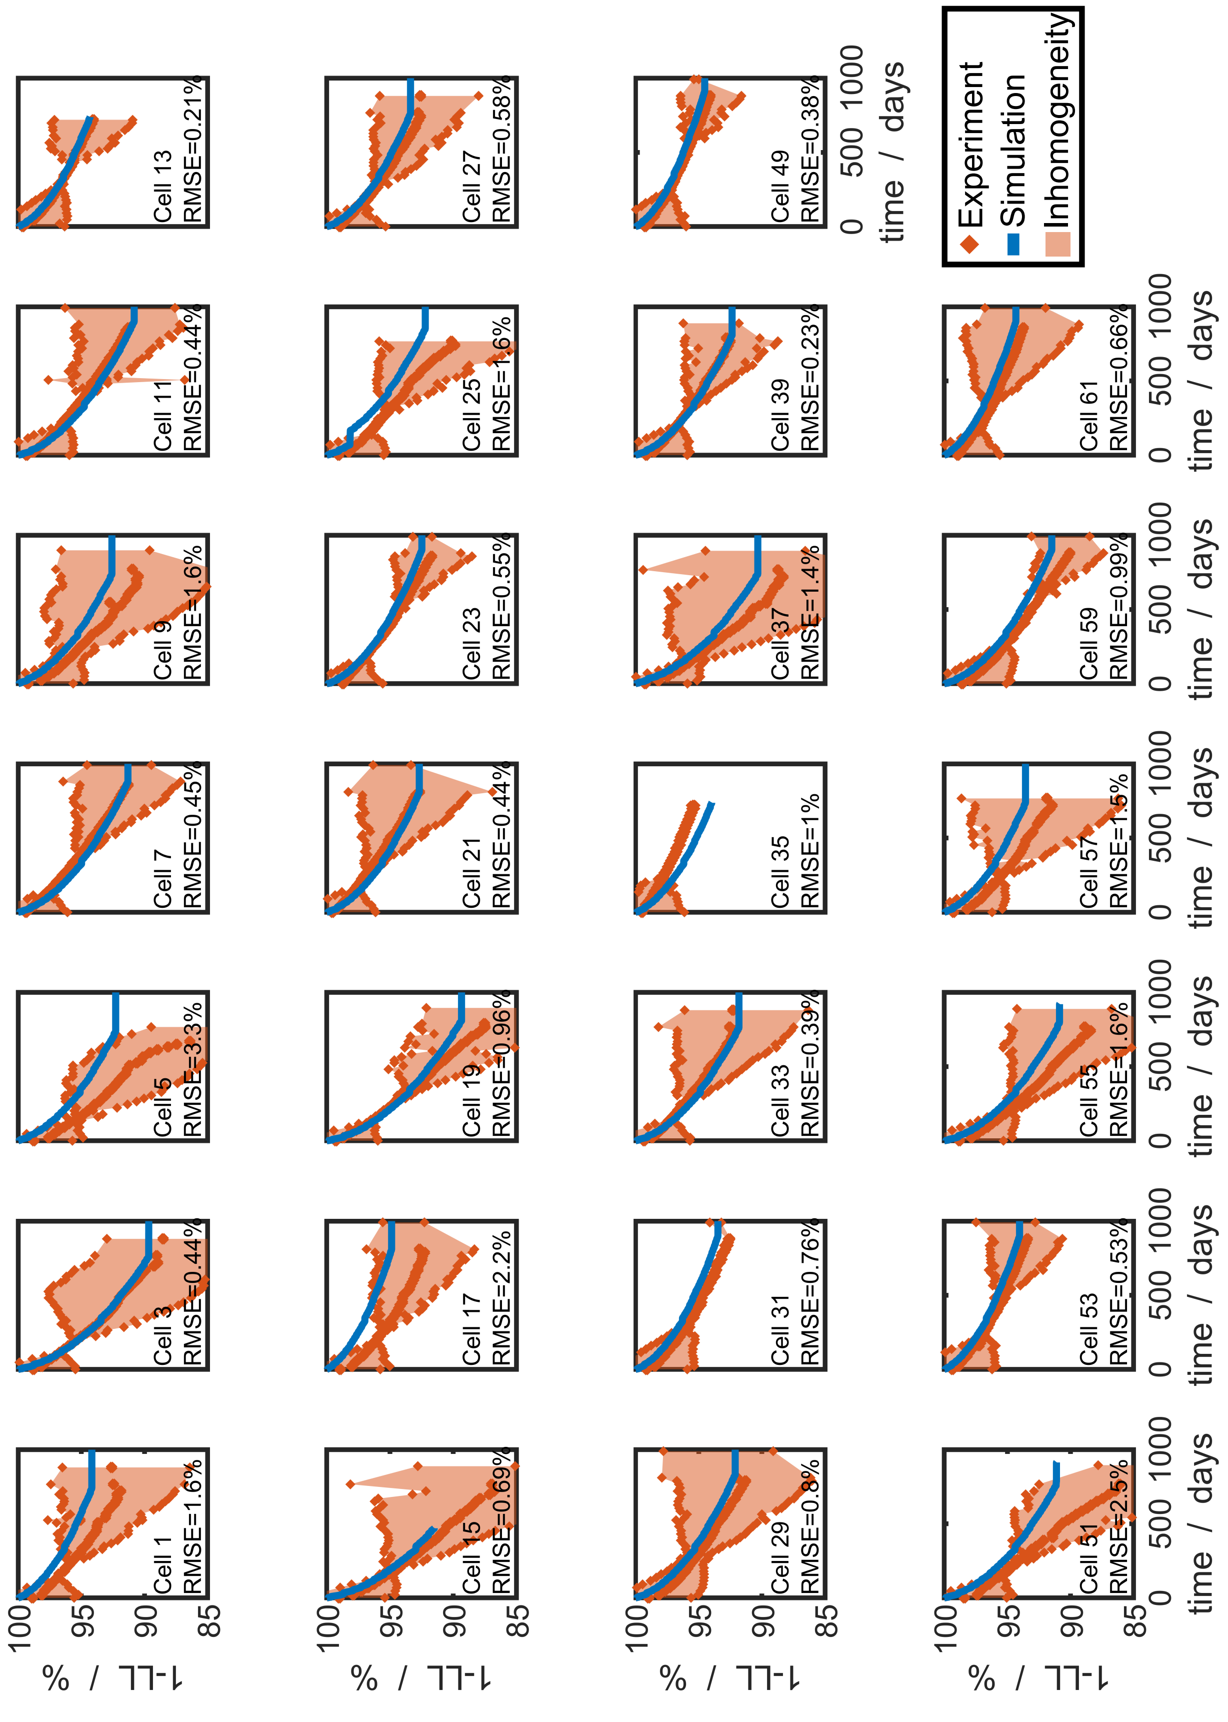


Figure SI-3: Complete model evaluation on the 28 different protocols.
